# Supplementary material for: To Err is Machine: Vulnerability Detection Challenges LLM Reasoning
Source: arXiv:2403.17218 source file (2025-01-07)
Supplement: Supplementary file 2 [file 99.findings-appendix.tex]

\section{Appendix: examples of our prompt templates}
\label{sec:prompt-examples}

\subsection{Legend}
\begin{itemize}
    \item \textcolor{\KeywordColor}{Gray} text represents sections of text which are excluded for brevity or conciseness.
    \item \textcolor{\HintColor}{Blue} text marks prompt hints which are inserted to condition the model's response. These can be in-context examples, or the ``hard-coded start'' of the model's completion. For example, in the Q/A prompt template, we append \texttt{\textcolor{\HintColor}{Answer:}} as a hard-coded start for the model's completion to influence its response to answer the question marked with \texttt{Question:}.
    \item \textcolor{\CompletionColor}{Green} text marks the area where the model will generate a completion.
\end{itemize}

\subsection{Basic prompt templates}

Here we list the prompt templates we used which do not incorporate any examples for in-context learning.
These queries can be used in $n$-shot prompts to boost the performance or induce a certain behavior from the model.

\begin{minipage}{\linewidth}\begin{lstlisting}[caption=Basic prompt template]
Is the following function buggy? Please answer Yes or No.
```
<@\textcolor{gray}{[Code]}@>
```
<@\textcolor{\CompletionColor}{[Completion]}@>
\end{lstlisting}\end{minipage}

\begin{minipage}{\linewidth}\begin{lstlisting}[caption=Basic template with system prompt]
<@\textcolor{\KeywordColor}{<SystemToken>}@>I want you to act as a vulnerability detection system.<@\textcolor{\KeywordColor}{</SystemToken>}@>
Is the following function buggy? Please answer Yes or No.
```
<@\textcolor{\KeywordColor}{[Code]}@>
```
<@\textcolor{\CompletionColor}{[Completion]}@>
\end{lstlisting}\end{minipage}

\begin{minipage}{\linewidth}\begin{lstlisting}[caption=CWE list query (all bug types in the dataset)]
Does the following function contain one of the following bug types? Please answer Yes or No.
- CWE-190: Integer Overflow
- CWE-476: Null Pointer Dereference
- CWE-125: Out-of-bound Read
- CWE-787: Out-of-bound Write
- CWE-416: Use After Free
```
<@\textcolor{\KeywordColor}{[Code]}@>
```
<@\textcolor{\CompletionColor}{[Completion]}@>
\end{lstlisting}\end{minipage}

\begin{minipage}{\linewidth}\begin{lstlisting}[caption=Q/A template]
Question: Is the following function buggy? Please answer Yes or No.
```
<@\textcolor{\KeywordColor}{[Code]}@>
```
<@\textcolor{\HintColor}{Answer:}@> <@\textcolor{\CompletionColor}{[Completion]}@>
\end{lstlisting}\end{minipage}

\subsection{$n$-shot prompt templates}

There are several dimensions to our design, which can affect the model's performance:
\begin{itemize}
    \item \textbf{From which dataset to select the examples?} We selected examples from the SVEN evaluation dataset (excluding the example in the query and its correponding buggy or fixed version), or from the BigVul or D2A datasets (as baselines for our CoT approaches which depend on these datasets). 
    \item \textbf{How to order the examples?} We have found that the model performs best when the order of the examples are randomly shuffled in the prompt template.
    We also experimented with placing vulnerable examples first, non-vulnerable examples first, or sorting by similarity score; in these strategies, the models may suffer from recency bias, as noted by \citet{prompting-bias}.
    \item \textbf{What is the distribution of labels in the examples?} We can adjust the distribution of labels to include more vulnerable or non-vulnerable examples. We found that a balanced distribution worked best in our experiments, possibly due to the majority label bias discussed in \citet{prompting-bias}.
    \item \textbf{How many examples are included in the context?} We experimented to find the best number of examples; the models generally performed better with more examples.
    \item \textbf{How are the examples selected?} In the basic version, we select examples randomly from the dataset.
    % The examples can be chosen by selecting randomly from the dataset, or similarity search using SentenceTransformers embedding, CodeBERT embedding, or OpenAI Babbage embedding~\cite{rag}.
    % \todo{TODO: How are the examples selected?}
\end{itemize} 

The in-context examples can be selected randomly, or by looking up the most similar code in a labeled dataset according to a similarity score.

We used this template to induce chain-of-thought responses by replacing the example responses in \textcolor{\HintColor}{blue} with chains of thought (shown below).

The hyphens \texttt{---} denote breaks between the example responses and subsequent queries.
For chat models, we sent each query and response to the model as a separate message in the appropriate role.

\begin{minipage}{\linewidth}\begin{lstlisting}[caption=$n$-shot prompt template]
Is the following function buggy? Please answer Yes or No.
```
<@\textcolor{\KeywordColor}{[Labeled Code 1]}@>
```
<@\textcolor{\HintColor}{Yes, the program is buggy.}@>
---
Is the following function buggy? Please answer Yes or No.
```
<@\textcolor{\KeywordColor}{[Labeled Code 2]}@>
```
<@\textcolor{\HintColor}{No, the program is not buggy.}@>
---
Is the following function buggy? Please answer Yes or No.
```
<@\textcolor{\KeywordColor}{[Unseen Code]}@>
```
<@\textcolor{\CompletionColor}{[Completion]}@>
\end{lstlisting}\end{minipage}

\subsection{Chain-of-thought from CWE Descriptions}
Example for in-context learning, sourced from \url{https://nvd.nist.gov/vuln/detail/CVE-2013-6051}:

\begin{minipage}{\linewidth}\begin{lstlisting}[caption=CoT-CVE in-context example]
Is the following function buggy? Please answer Yes or No.
```
<@\textcolor{\KeywordColor}{[Code]}@>
```
<@\textcolor{\HintColor}{The bgp\_attr\_unknown function in bgp\_attr.c in Quagga 0.99.21 does not properly initialize the total variable, which allows remote attackers to cause a denial of service (bgpd crash) via a crafted BGP update. Therefore, Yes, the program is buggy.}@>
\end{lstlisting}\end{minipage}

\subsection{Chain-of-thought from Static Analysis}
Example for in-context learning, sourced from hypothetical output from the Infer static analyzer~\citep{infer,d2a}:

\begin{minipage}{\linewidth}\begin{lstlisting}[caption=CoT-SA in-context example]
Is the following function buggy? Please answer Yes or No.
```
<@\textcolor{\KeywordColor}{[Code]}@>
```
<@\textcolor{\HintColor}{1. A buffer buf of size 10 is allocated at line 1.}@>
<@\textcolor{\HintColor}{2. An index i is initialized to a value in the range [0, 100] at line 2.}@>
<@\textcolor{\HintColor}{3. The index i is used to access buf at line 3. This may exceed the bounds of buf.
Therefore, Yes, the program is buggy.}@>
\end{lstlisting}\end{minipage}

\subsection{Chain-of-thought from Conversations}

This is an example of a conversation. The roles are annotated in \textcolor{\HintColor}{Blue} and \textcolor{\CompletionColor}{Green} at the top of each turn.

\begin{lstlisting}[caption=CoT-Conversation example]
<@\centering\textcolor{\HintColor}{[User]}@>
'''static gboolean prplcb_xfer_new_send_cb(gpointer data, gint fd, b_input_condition cond)
{
PurpleXfer *xfer = data;
	struct im_connection *ic = purple_ic_by_pa(xfer->account);
	struct prpl_xfer_data *px = xfer->ui_data;
	PurpleBuddy *buddy;
	const char *who;
	buddy = purple_find_buddy(xfer->account, xfer->who);
	who = buddy ? purple_buddy_get_name(buddy) : xfer->who;
	/* TODO(wilmer): After spreading some more const goodness in BitlBee,
	   remove the evil cast below. */
	px->ft = imcb_file_send_start(ic, (char *) who, xfer->filename, xfer->size); 
	px->ft->data = px;
	px->ft->accept = prpl_xfer_accept;
	px->ft->canceled = prpl_xfer_canceled;
	px->ft->free = prpl_xfer_free;
	px->ft->write_request = prpl_xfer_write_request;
	return FALSE;
}'''
First, analyze every line of the given code very carefully to answer the question. At which specific line of the given code the pointer can be a NULL? Please explain the reason.
---
<@\centering\textcolor{\CompletionColor}{[Assistant]}@>
In the given code, the pointer `buddy` can be `NULL` at line 10 (`buddy = purple_find_buddy(xfer->account, xfer->who);`). 

The reason is that the function `purple_find_buddy()` returns a pointer to a `PurpleBuddy` structure if the buddy is found, or `NULL` if the buddy is not found. If the buddy is not found for the given `xfer->account` and `xfer->who`, the `buddy` pointer will be assigned `NULL`.
---
<@\centering\textcolor{\HintColor}{[User]}@>
corrections: the pointer can be NULL at the following line of the given code:
  "px->ft = imcb_file_send_start(ic, (char *) who, xfer->filename, xfer->size)"
---
<@\centering\textcolor{\CompletionColor}{[Assistant]}@>
Apologies for the confusion. You are correct. The pointer `px->ft` can be `NULL` at the line:

```cpp
px->ft = imcb_file_send_start(ic, (char *) who, xfer->filename, xfer->size);
```

The reason is that the function `imcb_file_send_start()` may return a `NULL` pointer if there is an error or if the file transfer cannot be initiated for some reason. It is important to handle this possibility in the code to avoid potential issues when accessing `px->ft` later in the program.
---
<@\centering\textcolor{\HintColor}{[User]}@>
Now, based on the earlier conversation please answer which specific pointer of the above-mentioned code can be a NULL.
---
<@\centering\textcolor{\CompletionColor}{[Assistant]}@>
Based on the earlier conversation, the specific pointer in the given code that can be `NULL` is `px->ft`.
---
<@\centering\textcolor{\HintColor}{[User]}@>
At which one specific line of the above-mentioned code the null pointer is dereferenced?
---
<@\centering\textcolor{\CompletionColor}{[Assistant]}@>
In the given code, there is no specific line where a null pointer is dereferenced. However, it is important to note that if `px->ft` is `NULL` and an attempt is made to access its members or invoke its functions, it would result in a null pointer dereference error. Therefore, it is crucial to handle the case where `px->ft` is `NULL` to avoid such errors.
---
<@\centering\textcolor{\HintColor}{[User]}@>
corrections: the pointer is dereferenced at the following line of the given code: "px->ft->data = px;"
---
<@\centering\textcolor{\CompletionColor}{[Assistant]}@>
Apologies for the oversight. You are correct. The null pointer is dereferenced at the line:

```cpp
px->ft->data = px;
```

If `px->ft` is `NULL`, attempting to access its member `data` would result in a null pointer dereference error. It is important to ensure that `px->ft` is not `NULL` before accessing its members to avoid such errors.
---
<@\centering\textcolor{\HintColor}{[User]}@>
Now, first, analyze the earlier conversation. Can a NULL pointer "px->ft" be dereferenced in the above-mentioned program? Please answer as "Yes" or "No". Then explain the reason for your response
---
<@\centering\textcolor{\CompletionColor}{[Assistant]}@>
Yes, a NULL pointer `px->ft` can be dereferenced in the above-mentioned program.

The reason is that at the line `px->ft->data = px;`, if `px->ft` is NULL, attempting to access its member `data` would result in a null pointer dereference error. This means that if `imcb_file_send_start()` returns NULL or if `px->ft` is not assigned a valid value before this line, dereferencing `px->ft` would lead to undefined behavior. It is important to handle this possibility in the code to avoid such errors.
---
<@\centering\textcolor{\HintColor}{[User]}@>
First carefully analyze our entire earlier conversations like questions, answers, and corrections; then consider those to answer the question. Does this program contain any vulnerabilities? Please answer "Yes" or "No". Explain the reason and if your answer is Yes, then please mention the name of that vulnerability. if your answer is No, then please mention this is Non-Vulnerable
---
<@\centering\textcolor{\CompletionColor}{[Assistant]}@>
Based on our earlier conversations and analysis of the code, the program does contain a vulnerability.

The vulnerability is a potential null pointer dereference. This occurs at the line `px->ft->data = px;` where `px->ft` is assigned a value without checking if it is `NULL`. If `px->ft` is `NULL`, attempting to access its member `data` would result in a null pointer dereference error.

To address this vulnerability, it is important to add a check to ensure that `px->ft` is not `NULL` before dereferencing it.
\end{lstlisting}


\section{Appendix: Metrics with more details}
